# Supplementary material for: Improving the Privacy and Practicality of Objective Perturbation for Differentially Private Linear Learners
Source: arXiv:2401.00583 source file (2023-12-31)
Supplement: Supplementary file 1 [file distributed.tex]

\section{Objective perturbation in a distributed setting}\:
In real-world deployment, computing resources are often distributed across many devices which don't share data. For differentially private learning in this setting, the usual approach is to switch to a local DP (LDP) model in which each user holds her own data and adds noise to it locally.

% {\color{blue} The following paragraph is a bit confusing, because it claims that the data is accessed only through the gradients. This is true if we use SGD, but not necessarily true for any blackbox optimizer.}

While objective perturbation can't traditionally operate in combination with the LDP model -- as it requires a centralized database -- Algorithm~\ref{alg:comp_objpert} could readily extend to a distributed setting. Suppose we use a first-order optimizer such as SGD; then data is accessed only through the gradients $\nabla \ell(\theta; z)$. In this case, the key difference between the objective perturbation step of Algorithm~\ref{alg:comp_objpert} and DP-SGD is that ObjPert adds the \emph{same} noise $b$ (scaled according to the batch size $n_B$) at each iteration, rather than sampling fresh noise every time. Since Gaussian-distributed random variables are closed under addition (i.e., the sum of two Gaussians is a Gaussian), we can sample $b \sim \mathcal{N}(0, \sigma^2I_d)$ in a distributed fashion: at iteration $i \in [n]$, user $i$ adds $b_i \sim \mathcal{N}(0, \frac{\sigma^2}{n}I_d)$ to her data $\nabla \ell(\hat{\theta}^P_i; z_i)$. The noise scale could also be adjusted to accommodate multiple passes over the dataset.

We can also connect Algorithm~\ref{alg:comp_objpert} to \emph{differentially private follow-the-regularized-leader} (DP-FTRL) \citep{kairouz2021practical}, which uses a tree-based aggregation algorithm to privately release the gradients of the loss function as a prefix sum. This approach provides a competitive privacy/utility tradeoff without relying on privacy amplification or shuffling, which is often not possible in distributed settings. DP-FTRL differs from DP-SGD by adding \emph{correlated} rather than \emph{independent} noise at each iteration; Algorithm~\ref{alg:comp_objpert}, in contrast, differs from both by adding \emph{identical} noise at each iteration.
