# Supplementary material for: Improving the Privacy and Practicality of Objective Perturbation for Differentially Private Linear Learners
Source: arXiv:2401.00583 source file (2023-12-31)
Supplement: Supplementary file 2 [file additional_background.tex]

\subsection{Convex Optimization}
We give a short review of relevant concepts from convex optimization.
\begin{definition}[$\ell_2$-Lipschitz continuity]
\label{defn:lipschitz_continuity}
A function $f: \Theta \rightarrow \mathbb{R}$ is $L$-Lipschitz w.r.t. the $\ell_2$-norm over $\Theta \subseteq \mathbb{R}^d$ if for all $\theta_1, \theta_2 \in \Theta$, the following holds: $|f(\theta_1) - f(\theta_2)| \leq L|| \theta_1 - \theta_2||_2.$
\end{definition}

\begin{definition}[$\beta$-smoothness]
\label{defn:beta_smoothness}
A differentiable function $f: \Theta \rightarrow \mathbb{R}$ is $\beta$-smooth over $\Theta \subseteq \mathbb{R}^d$ if its gradient $\nabla f$ is $\beta$-Lipschitz, i.e. $|\nabla f(\theta_1) - \nabla f(\theta_2)| \leq \beta|| \theta_1 - \theta_2||_2$ for all $\theta_1, \theta_2 \in \Theta$.
\end{definition}

\begin{definition}[Strong convexity]
\label{defn:strong_convexity}
A differentiable function $f: \Theta \rightarrow \mathbb{R}$ is $\lambda$-strongly convex over $\Theta \subseteq \mathbb{R}^d$ if for all $\theta_1, \theta_2 \in \Theta$: $f(\theta_1) \geq f(\theta_2) + \nabla f(\theta_2)^T (\theta_1 - \theta_2) + \frac{\lambda}{2}||\theta_1 - \theta_2 ||_2^2.$
\end{definition}

\subsection{RDP discussion}

Pure DP ($\delta= 0$) guarantees a bound $\epsilon$ on the privacy loss. Approximate DP ($\delta > 0$) implies a high-probability bound on the privacy loss: By allowing a privacy breach (arbitrarily large $\epsilon$) to occur with a small probability $\delta$, we can often get a tighter characterization of the privacy loss.

RDP gives a tighter characterization of the privacy loss, without risking an arbitrarily large privacy breach.

RDP is often viewed as an ideal middle ground between pure DP and approximate DP. Approximate DP allows an arbitrarily large privacy breach to happen with some small probability; RDP avoids this catastrophic failure possibility by enforcing a bound in \emph{expectation} (averaging across all outputs of a mechanism) on the $\alpha$-th moment of the privacy loss random variable. Compared to pure DP, RDP provides tighter privacy composition and is thus well-suited to the analysis of DP-SGD, which invokes the (subsampled) Gaussian mechanism over many iterations.

\subsection{Privacy Loss Random Variables}

\begin{lemma}[PLRV of Gaussian mechanism \citep{balle2018improving}]
\label{lemma:plrv_gaussian}
    The privacy loss random variable of the Gaussian mechanism $\mathcal{M}(Z) = f(Z) + \mathcal{N}(0, \sigma^2 I_d)$ for a function $f: \mathcal{Z} \rightarrow \mathbb{R}^d$ and neighboring datasets $Z, Z'$ follows a Gaussian distribution $\mathcal{N}\left(\dfrac{\Delta_{Z, Z'}^2}{2\sigma^2}, \dfrac{\Delta_{Z, Z'}^2}{\sigma^2}\right)$, where $\Delta_{Z, Z'} = ||f(Z) - f(Z')||_2$.
\end{lemma}
