# Supplementary material for: Improving the Privacy and Practicality of Objective Perturbation for Differentially Private Linear Learners
Source: arXiv:2401.00583 source file (2023-12-31)
Supplement: Supplementary file 3 [file beta_preservation.tex]

\section{Clipping the Gradients Preserves Lipschitz-smoothness}

Proving Theorem~\ref{thm:rdp_alg1} (the privacy guarantee of Algorithm~\ref{alg:comp_objpert}) will require proving several properties of the ``clipped-gradient'' function $\ell_C(\theta; z)$:

\begin{enumerate}
    \item We need to show that the ``clipped-gradient'' function $\ell_C(\theta; z)$ retains the  convex GLM structure of the original function $\ell(\theta; z)$.
    \item We need to show that the ``clipped-gradient'' function $\ell_C(\theta; z)$ satisfies $||\nabla \ell_C(\theta; z)||_2 \leq C$ for any $\theta, z$.
    \item We need to show that the ``clipped-gradient'' function $\ell_C(\theta; z)$ has the same $\beta$-smoothness parameter as the original function $\ell(\theta; z)$.
\end{enumerate}

 We will begin by stating a result from \citet{song2020evading}.

\begin{theorem}[{\citealp[Lemma 5.1]{song2020evading}}]
\label{thm:characterizing_clipped_gradient}
    Let $f: \mathbb{R} \rightarrow \mathbb{R}$ be any convex function and let $C \in \mathbb{R}_{+}$ be any positive value. For any non-zero $x \in \mathbb{R}^d$, define 
    \begin{align*}
        U_L &= \left\{ u : g < - \frac{C}{||x||_2 }\:\:\:\forall g \in \partial f(u)\right\}, \\
        U_H &= \left\{ u : g > \frac{C}{||x||_2 } \:\:\:\forall g \in \partial f(u)\right\}.
    \end{align*}
    If $U_L$ is non-empty, let $u_L = \sup U_L$; otherwise $u_L = -\infty$. If $U_H$ is non-empty, let $u_H = \inf U_H$; otherwise $u_H = \infty$. For any non-zero $x \in \mathbb{R}^d$, let
    \begin{align*}
        f_C(u) &= \begin{cases}
			-\frac{C}{||x||_2}\left(u - u_L \right), & \text{for $u \in (-\infty, u_L)$}\vspace{3pt}\\
   f(u; y), & \text{for $u \in (u_L, u_H)$}\vspace{3pt}\\
   \frac{C}{||x||_2}\left(u - u_H \right), & \text{for $u \in (u_H, \infty)$}
		 \end{cases}
    \end{align*}
    Define $u_x(\theta) = x^T \theta$. Then the following holds.
    \begin{enumerate}
        \item $f_C$ is convex.
        \item Let $\ell(\theta; (x, y)) = f(u_x(\theta); y)$ for any $\theta, z = (x, y)$. Then we have
        \begin{align*}
            \partial_{\theta} \ell_C(\theta; z) &= \left\{ \min\left\{1, \frac{C}{||u_x(\theta)||_2)}\right\} \cdot u : u \in   \partial_{\theta} \ell(\theta; z) \right\}.
        \end{align*}
    \end{enumerate}
\end{theorem}

The first two desired properties of $\ell_C(\theta; z)$, i.e. GLM structure and gradient norm bound $C$, follow directly from the above theorem. Next, we will prove the third property of $\beta$-smoothness.

\begin{theorem}
For a data point $z = (x, y)$, consider a function $f$ such that $\ell(\theta; z) = f(x^T\theta; y)$. Suppose that $f(x^T\theta; y)$ satisfies $\beta$-smoothness. Then the ``clipped-gradient'' function $f_C(x^T\theta; y)$ defined in Lemma 5.1 of \citet{song2020evading} also satisfies $\beta$-smoothness.
\end{theorem}

\begin{proof}
Because $f$ is $\beta$-smooth by assumption, we know that the following holds for all $u_1, u_2 \in $
\end{proof}
