# Supplementary material for: Improving the Privacy and Practicality of Objective Perturbation for Differentially Private Linear Learners
Source: arXiv:2401.00583 source file (2023-12-31)
Supplement: Supplementary file 4 [file errata.tex]

\section{Errata}

\subsection{Excess Empirical Risk}

In the statement of Theorem~\ref{thm:excess_emp_risk}, we omitted the term $\frac{\lambda}{2}||\theta^*||_2^2$ and also didn't provide a tight bound on the expectation of the norm of the noise vector $b_2 \sim \mathcal{N}(0, \sigma_{out}^2I_d)$. In the appendix we have fixed this, and the revised bound on excess empirical risk for Algorithm~\ref{alg:comp_objpert} is
\begin{align*}
    \mathbb{E} \left[ \mathcal{L}(\Tilde{\theta}^P; Z) \right] - \mathcal{L}(\theta^*; Z) &\leq nL \left(\frac{\tau}{\lambda}+  \sigma_{out}\sqrt{d} \right) + \frac{(n\beta||\mathcal{X}||_2^2 + \lambda)d\sigma^2}{2\lambda^2} + \frac{\lambda}{2}||\theta^*||_2^2.
\end{align*}

\subsection{Assumptions on the loss function}
In the main paper we have assumed that $\nabla^2 \ell(\theta; z) \prec \beta I_d$, i.e. $\ell(\cdot)$ is $\beta$-smooth. However for results specific to GLM-structured losses (e.g., Theorem~\ref{thm:rdp_objpert}), we require the slightly stronger assumption that $f$ is $\beta$-smooth, where $\ell(\theta; z) = f(x^T \theta; y)$.
